# Supplementary material for: Galaxy Morphology in CANDELS: Addressing Evolutionary Changes Across $0.2 \leq z \leq 2.4$ with Hybrid Classification Approach
Source: arXiv:2412.03778 source file (2025-01-23)
Supplement: Supplementary file 1 [file section_appendix_hst_smooth.tex]

\section{}\label{sec:appendix1}
TEXT
